# Supplementary material for: Iterative Random Forests to detect predictive and stable high-order interactions
Source: arXiv:1706.08457 source file (2017-12-23)
Supplement: Supplementary file 1 [file supp-housing.tex]

\section{Case Study III: Ames Housing Sales} \label{sec:housing}

The iRF algorithm was motivated primarily by biological problems, but we anticipate that it will be a useful tool for interpreting feature interactions in other areas as well. In this section, we consider a dataset containing $80$ features on $2930$ sales of
residential property in Ames, Iowa between 2006 and 2010 (\href{http://ww2.amstat.org/publications/jse/v19n3/Decock/AmesHousing.txt}{http://ww2.amstat.org/}). The straightforward interpretation of features from this dataset provides an interesting and intuitive test case for exploring interactions recovered by iRF. We note that
for this regression problem, we sample from all leaf nodes in our generalized RIT instead of sampling from a class specific subset as in the enhancer and splicing data. As a result, recovered interactions represent features that collectively determine home value, whether low or high.

Of the $80$ features included in the Ames dataset, several were not recorded for
a large number of housing sales. We removed any feature for which more than
$100$ sales were missing data as well as observations with any missing features
following this step, leaving a total of $2826$ sales and $70$ features
(including sale price). In addition to features that were missing data, several
contained redundant information, particularly those related to area (sqft) in
different parts of a home. We combined measurements of ``livable'' area into a
single variable that included first story, second story, and finished basement
total area (sqft) and removed variables containing different aggregate
measurements of above and below ground area. After setting aside sale price as
the response of interest, we were left with a total of $64$ features.

We randomly divided the data into training and test sets of size $2119$
($75\%$) and $707$ ($25\%$) and ran iRF with $K=3$ and $B=20$. We set RF
parameters to the standard \texttt{R} \texttt{randomForest} values, and grew
$M=100$ random intersections trees of depth $5$ with $n_{child}=2$. Each of the
three iRF iterations $K=1,2,3$ achieved comparable predictive performance,
explaining $88.9\%, 88.1\%,$ and $88.0\%$ of the variance in sale prices
respectively. 

The interactions recovered by iRF are shown in Figure \ref{fig:irf-housing}A.
Unsurprisingly, overall quality is particularly important for predicting sale
price. This ordinal feature provides an aggregate rating of the overall material
and finish of a home that ranges from very poor (1) to very excellent (10).
Most of the interactions identified by iRF encode relationships between overall
quality and other features of the house (e.g. livable square footage, year
built, lot area). 

We investigated the relationship between overall quality and other features and
found that homes rated higher for overall quality exhibit
different sale price behavior than homes rated lower for overall quality.
Figures \ref{fig:irf-housing}B,C show response surfaces of two third order
interactions recovered by iRF that demonstrate these differences. The response surfaces for livable
area (sqft), lot size (sqft), and sale price (Figure \ref{fig:irf-housing}B)
indicates that there is a stronger association between lot size and sale price,
relative to the association between livable area and sale price, in lower
quality homes than in higher quality homes. This finding would suggest that for
lower quality homes, land plays a bigger role in final sale price. The response
surfaces for livable area (sqft), year built, and sale price (Figure
\ref{fig:irf-housing}C) shows that the sale price of high quality homes appears
to be fairly independent of year built. In contrast, lower quality homes of
comparable size have a stronger association between sale price and year built.

%iRF also recovers interactions that appear reflect boolean-type relationships between features. For instance, Figure \ref{fig:irf-housing}B shows the relationship between livable area, garage area, and sale price. The average sale price of houses in $80^{th}$ percentile of both livable and garage square footage is more than $135\%$ of the sale price of houses falling in the $80^{th}$ percentile for only one of these variables. In comparison, moving up one quantile for one of these variables, with the other variable held fixed, on average only results in a $113\%$ increase in predicted price in other regions of the feature space.
